# Supplementary material for: Possible Realization of Kitaev Spin Liquids in van der Waals Heterostructures of $\alpha$-RuCl$_3$ and Cr$X_3$ ($X$=Cl and I)
Source: arXiv:2310.01075 source file (2024-12-25)
Supplement: Supplementary file 1 [file SM.pdf]

# Supplemental Material for Possible Realization of Kitaev Spin Liquids in van der Waals Heterostructures of $\alpha$-RuCl$_3$ and Cr$X_3$ ($X$=Cl and I)

Lingzhi Zhang and Yukitoshi Motome
*Department of Applied Physics, The University of Tokyo, Bunkyo, Tokyo 113-8656, Japan*
(Dated: November 18, 2024)

## S1. Magnetic anisotropy in $\alpha$-RuCl$_3$/CrCl$_3$ and $\alpha$-RuCl$_3$/CrI$_3$

We calculate the magnetic anisotropy energy for two heterostructures, $\alpha$-RuCl$_3$/CrCl$_3$ and $\alpha$-RuCl$_3$/CrI$_3$, by rotating the Cr moment from the most stable magnetic states obtained in the main text. The results for $\alpha$-RuCl$_3$/CrCl$_3$ are shown in Fig. S1 by rotations within (a) the $ab$ plane and (b) the $ac$ plane. In this case, the magnetic anisotropy in the CrCl$_3$ layer is less than 1 meV, indicating that the AFM interlayer interaction is in the order of 0.1 meV.

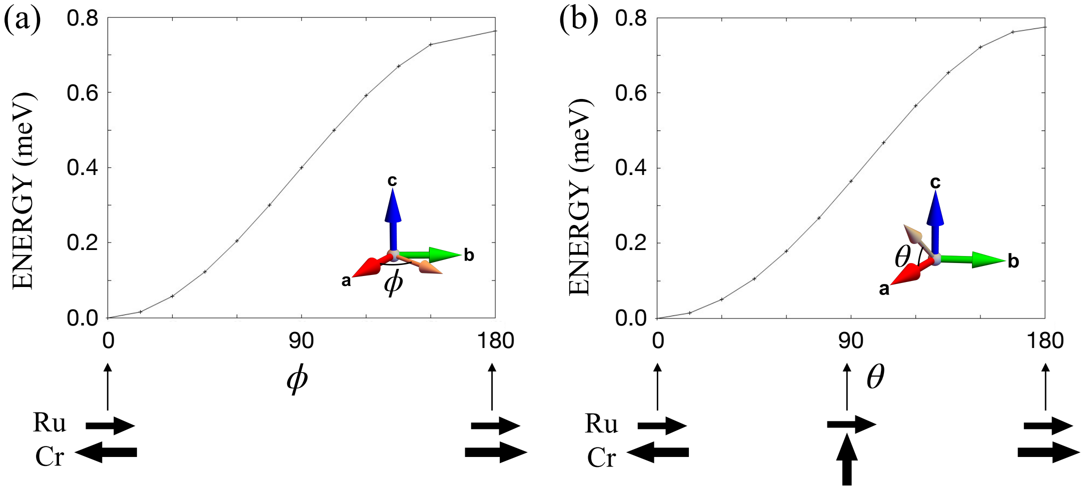


FIG. S1. Magnetic anisotropy energy in the CrCl$_3$ layer of $\alpha$-RuCl$_3$/CrCl$_3$ for the rotations of the Cr moment within (a) the $ab$ plane and (b) the $ac$ plane. The Ru moments are fixed along the $-a$ axis. The insets denote the definitions of the angles $\theta$ and $\phi$. Schematics of the arrangements of Ru and Cr moments are shown below each panel.

Figure S2 shows the results for $\alpha$-RuCl$_3$/CrI$_3$. In this case, the magnetic anisotropy in the CrI$_3$ layer is about 3 meV, indicating that the interlayer interaction is also AFM but the strength is one order of magnitude larger than that in $\alpha$-RuCl$_3$/CrCl$_3$. Nonetheless, the most stable is not the interlayer AFM state but the state with the Cr moment canted by about 30 degrees from the $c$ axis, presumably due to the strong out-of-plane anisotropy existing in the CrI$_3$ monolayer.

## S2. Exact diagonalization calculation for 24-site cluster

We perform the exact diagonalization calculations for the spin Hamiltonian in Eq. (1) in the main text with the estimates of exchange constants in Table III. Following the prior work [2], we consider a 24-site cluster with the periodic boundary condition, and adopt the H$\Phi$ package to conduct our calculations using the Lanczos algorithm [3, 4].

Figure S3 shows the results of spin structure factor $S(\boldsymbol{q})$ at the $M$ point in the first Brillouin zone (red), which signals the zigzag order, and the uniform magnetic moment per spin, $m$ (black), under in-plane magnetic fields with the $g$-factor of 2.4 [5]. For the heterostructure of $\alpha$-RuCl$_3$ and CrCl$_3$, we observe rapid suppression of the zigzag order with the in-plane magnetic field of $\sim$ 25 T, where the induced magnetic moment reaches $\sim 0.7\ \mu_B$, as shown in Fig. S3(a). Although the value of the magnetic field is larger than the experimental one, the result agrees well with our claim that the heterostructure $\alpha$-RuCl$_3$/CrCl$_3$ possibly realizes the spin liquid regime where the zigzag order is suppressed in bulk. We believe that the discrepancy of the critical magnetic field is due to the small size cluster as well as the uncertainty of model parameters. For comparison, we also perform the calculations for bulk $\alpha$-RuCl$_3$ using the parameters in Table III of Ref. [1]. In this case, we observe similar results with the suppression of zigzag order

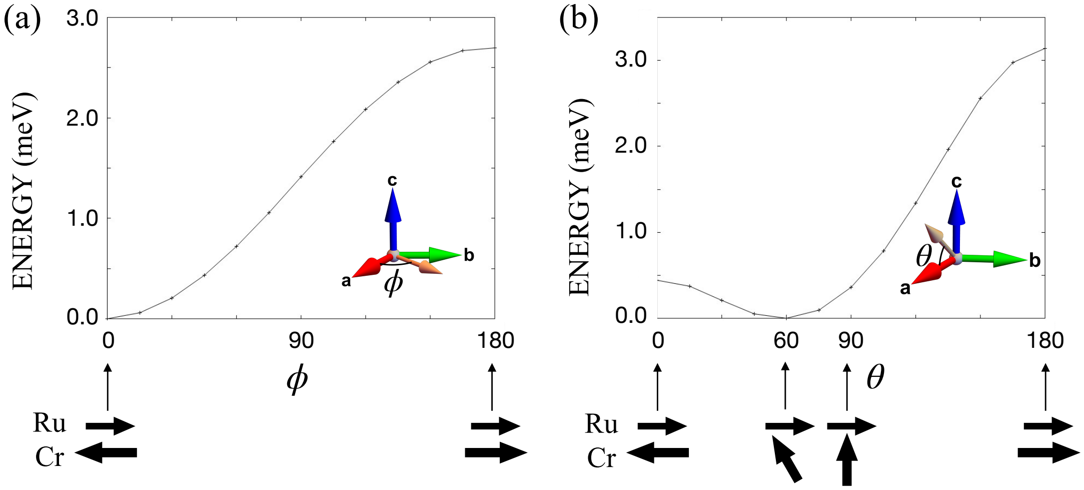


FIG. S2. Corresponding data for $\alpha$-$RuCl_3$/$CrI_3$. The notations are common to those in Fig. S1.

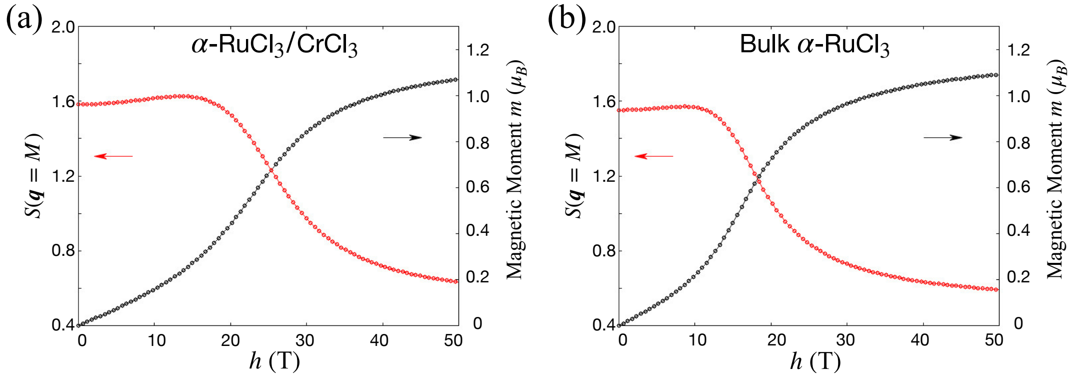


FIG. S3. Spin structure factor $S(\boldsymbol{q})$ at the $M$ point in the first Brillouin zone (red), and the magnetic moment per spin, $m$ (black), as functions of the in-plane magnetic field $h$ for the spin Hamiltonian in Eq. (1) in the main text with the estimated exchange constants of (a) the heterostructure of $\alpha$-$RuCl_3$ (see Table III in the main text) and (b) bulk $\alpha$-$RuCl_3$ in (see Table III in Ref. [1]).

with the in-plane magnetic field, but at a smaller magnetic field of $\sim 18$ T, as shown in Fig. S3(b). We note that the value of the critical field is also considerably larger than the experimental one, demonstrating the sensitivity to the cluster size and the model parameters.


[1] S. M. Winter, Y. Li, H. O. Jeschke, and R. Valentí, Challenges in design of Kitaev materials: Magnetic interactions from competing energy scales, Phys. Rev. B **93**, 214431 (2016).

[2] S.-H. Jang, Y. Kato, and Y. Motome, Vortex creation and control in the Kitaev spin liquid by local bond modulations, Phys. Rev. B **104**, 085142 (2021).

[3] K. Ido, M. Kawamura, Y. Motoyama, K. Yoshimi, Y. Yamaji, S. Todo, N. Kawashima, and T. Misawa, Update of HΦ: Newly added functions and methods in versions 2 and 3, Computer Physics Communications **298**, 109093 (2024).

[4] M. Kawamura, K. Yoshimi, T. Misawa, Y. Yamaji, S. Todo, and N. Kawashima, Quantum lattice model solver HΦ, Computer Physics Communications **217**, 180 (2017).

[5] R. D. Johnson, S. C. Williams, A. A. Haghighirad, J. Singleton, V. Zapf, P. Manuel, I. I. Mazin, Y. Li, H. O. Jeschke, R. Valentí, and R. Coldea, Monoclinic crystal structure of $\alpha$-$RuCl_3$ and the zigzag antiferromagnetic ground state, Phys. Rev. B **92**, 235119 (2015).
